# Supplementary material for: Modelling and predicting the effect of social distancing and travel restrictions on COVID-19 spreading
Source: arXiv:2010.05968 source file (2020-12-16)
Supplement: Supplementary file 1 [file SI.pdf]

# SUPPLEMENTARY INFORMATION for: Modelling and predicting the effect of social distancing and travel restrictions on COVID-19 spreading

Francesco Parino[1], Lorenzo Zino[2], Maurizio Porfiri[3], Alessandro Rizzo[1,4]

October 30, 2020

[1]Department of Electronics and Telecommunications, Politecnico di Torino, 10129 Turin, Italy
[2]Faculty of Science and Engineering, University of Groningen, 9747 AG Groningen, Netherlands
[3]Department of Mechanical and Aerospace Engineering and Department of Biomedical Engineering, New York University Tandon School of Engineering, Brooklyn NY 11201, USA
[4]Office of Innovation, New York University Tandon School of Engineering, Brooklyn NY 11201, USA

Correspondence should be addressed to: alessandro.rizzo@polito.it, mporfiri@nyu.edu

# Contents

**S1 Italian geographic organisation** **3**

**S2 Road map of NPIs in Italy** **5**

**S3 Details of the non-negative matrix factorisation (NMF)** **7**

**S4 Application of NMF to the analysis of mobility restrictions** **8**

**S5 Further details on the uplifting timing of NPIs** **10**

**S6 NMF to analyse the uplifting of mobility restrictions** **12**

**S7 Additional supporting simulations and figures** **14**

**Supplementary references** **18**

# S1 Italian geographic organisation

The Italian territory is divided into four levels of administrative entities. At the finer level, there are 7, 903 municipalities (local administrative units according to the European standards of Nomenclature of Territorial Units for Statistics - NUTS) that are grouped in 107 Provinces (NUTS-3). Provinces are then organised in 20 Regions (NUTS-2), which comprise five macro-regions (NUTS-1): *North-West*, *North-East*, *Centre*, *South* and *Islands*. See Fig. S1 for a map. We considered Provinces as the communities of our meta-population model. Such a choice has two main motivations. First, municipalities are not autonomous entities, since most of them are small and may not be able to provide all the necessary basic services to the population (supermarkets, hospitals, public offices, etc.). Hence, it could be unrealistic to propose that they are completely isolated with respect to the epidemic. Second, Provinces are the smallest administrative entities for which epidemic data can be considered consistently accurate and equally detailed nationwide.

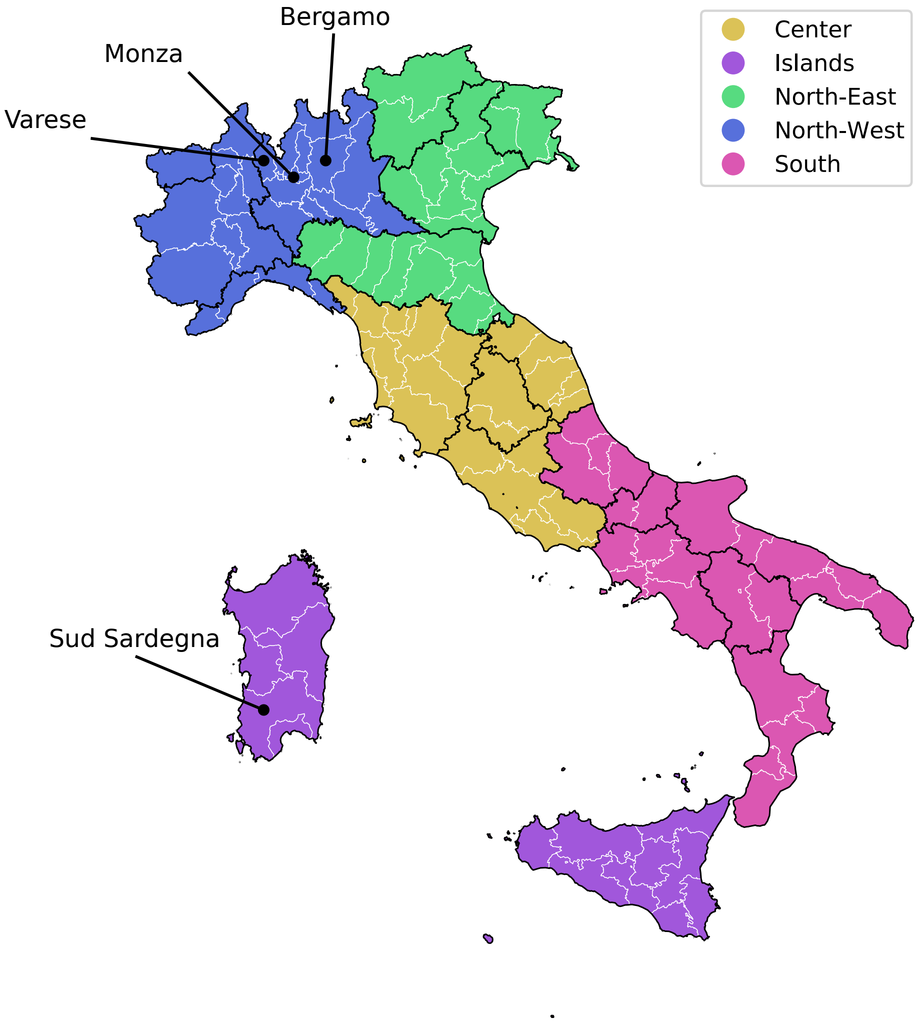


Figure S1: Administrative entities of Italy. The country is divided into 5 macro-regions, denoted by different colours in the figure. Macro-regions are divided into 20 Regions (separated by black outlines), which are partitioned into 107 Provinces (separated by white outlines). The Provinces used in the main document (*Bergamo*, *Monza*, *Sud Sardegna* and *Varese*) are labelled.

## S2 Road map of NPIs in Italy

- 20th–23rd February 2020: seven deaths are registered due to COVID-19, but they were not reported in [1], which starts reporting data from 24th February. These deaths are reported in the following news articles (in Italian):
  - https://www.agi.it/cronaca/news/2020-02-24/coronavirus-italia-7190713
  - https://www.adnkronos.com/fatti/cronaca/2020/02/24/coronavirus-tre-morti-italia_pGiCwRQVUyb3fisOFs027K.html
  - https://www.tgcom24.mediaset.it/cronaca/lombardia/coronavirus-morta-una-donna-in-lombardia-seconda-vittima-italiana_15150431-202002a.shtml
  - https://www.ilfattoquotidiano.it/2020/02/22/adriano-trevisan-78-anni-di-vo-euganeo-ecco-chi-e-la-prima-vittima-italiana-del-coronavirus-la-paura-nel-paese-isolato/5713686
  - https://www.ansa.it/canale_saluteebenessere/notizie/sanita/2020/02/24/coronavirus-_60aae600-8535-44d9-86de-48c4b71478ef.html
  - https://www.repubblica.it/cronaca/2020/02/23/news/coronavirus_italia-249329434/
- 21st–23rd February 2020: lockdown is enforced in the so called "red zones," areas around two municipalities in North Italy (*Codogno* in

*Lombardy* and *Vo'* in *Veneto*, located in *North-West* and *North-East* macro-regions, respectively).

- 1st March 2020: mild social distancing measures are enforced in large areas of *North-West* and *North-East*.
- 8th March 2020: strict lockdown is enforced in *Lombardy* and parts of *Veneto*, *Piemonte*, *Marche*; mild social distancing measures are extended to the entire country.
- 11th March 2020: severe lockdown, including activity reduction and mobility restrictions is extended nationwide.
- 18th May 2020: first relaxation of NPIs. Mitigation of the mobility restrictions (travels within the same Region are allowed) and partial reopening of commercial and productive activities.
- 3rd June 2020: complete relaxation of the mobility restrictions.
- 11th June 2020: further relaxation of NPIs.

All these interventions are recorded in the *Gazzetta Ufficiale della Repubblica Italiana* (Official Gazette of the Italian Republic) [2].

# S3 Details of the non-negative matrix factorisation (NMF)

Here, we explain the non-negative matrix factorisation (NMF) through the scenario of early implementations of NPIs, whose results are shown in Fig. S2. We simulated the total number of deaths, over a 104 days time-window, for $p$ different levels of $\alpha$, $q$ different levels of $\beta$, and for each Province $h \in \mathcal{H}$. The results of these simulations were stored in a set of non-negative matrices $P_h \in \mathbb{R}_+^{p \times q}$.

The NMF algorithm approximates each matrix $P_h$ as a weighted sum of an arbitrary number of basis matrices, which help understand the effect of NPIs on all the Provinces. We select two basis matrices, denoted as $C_1$ and $C_2$, so that

$$P_h \approx k_{h1} C_1 + k_{h2} C_2, \tag{1}$$

where $k_{h1}$ and $k_{h2}$ are two scalar weights that are specific to each matrix $P_h$.

The identification of both weights and basis matrices is performed through the following steps. First, we normalise the entries of each matrix $P_h$ between 0 and 1. Then, we assemble a new matrix $A \in \mathbb{R}_+^{|\mathcal{H}| \times (pq)}$, containing the vectorised of matrix $P_h$ at row $h$. Third, we minimise the residual in the Frobenius norm $||A - KH||_F$ to calculate matrices $K \in \mathbb{R}_+^{|\mathcal{H}| \times 2}$ and $H \in \mathbb{R}_+^{2 \times (pq)}$. The two row vectors of matrix $H$ contain the two basis matrices $C_1$ and $C_2$ in form of vectors, and the row vector $h$ of matrix $K$ comprises the two weights $k_{h1}$ and $k_{h2}$.

# S4 Application of NMF to the analysis of mobility restrictions

The application of the approach is presented in Fig. S2. As an illustration, we examine Fig. S2e-S2f that details further Fig. 6(c,f) of the main document. From Fig. S2e, we register that matrix $C_2$ encapsulates the beneficial effect of mobility restrictions, since the numerical value of its entries reflect the evidence that decreasing $\beta$ from 1 (no mobility restrictions) to 0 (no mobility allowed) results in a remarkable decrease in the number of deaths. On the contrary, matrix $C_1$ is associated with all the non-beneficial effects of mobility restrictions. We remark that, by construction, the NMF yields the two matrices $C_1$ and $C_2$ equal for all the Provinces. Hence, the relative magnitude of the two coefficients $k_{h1}$ and $k_{h2}$ indicates whether a given Province is benefited or harmed by mobility restrictions. Fig. S2f plots the coefficient pairs $(k_{h1}, k_{h2})$, for each Province. To provide a more illustrative evidence, a 2-means clustering algorithm [3] is applied to partition all Provinces in two sets: those for which mobility restrictions are beneficial and those for which they are detrimental. More details on the exemplary Provinces of *Sud Sardegna* and *Bergamo* (explicitly labelled in Fig.S2f) are presented in Fig. 6(c,f) of the main document. The other panels of Fig. S2 demonstrate analogous results for different dates of applications of NPIs, for which the effect of mobility restrictions is less evident.

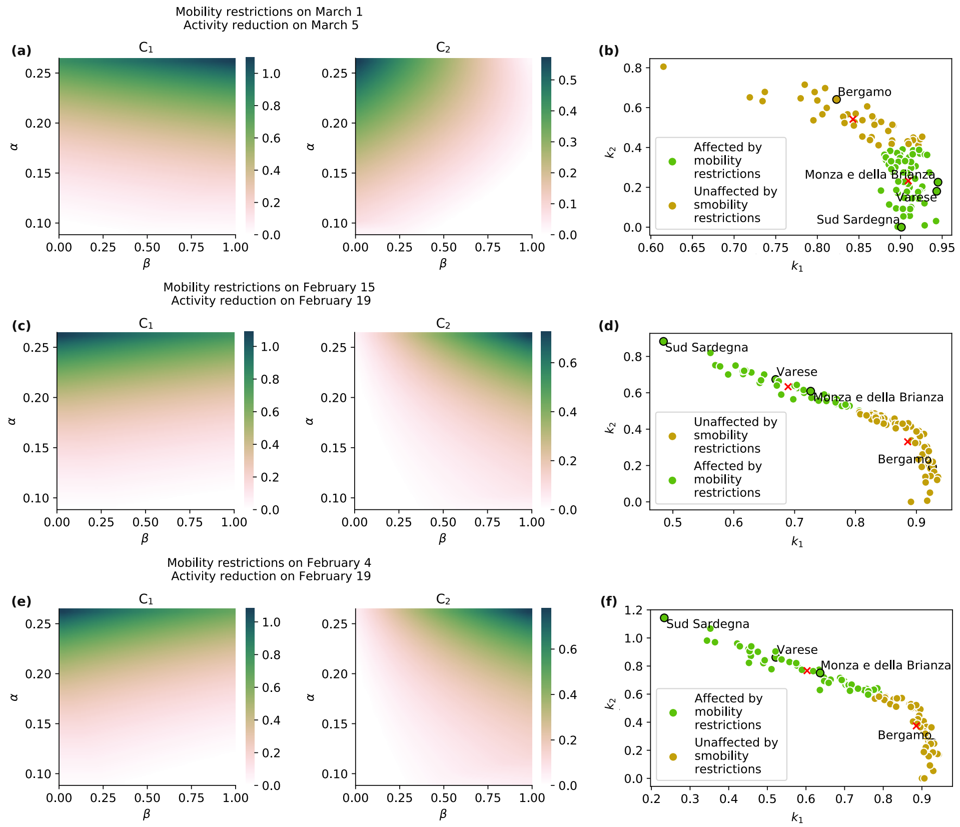


Figure S2: Effect of activity reduction and mobility restrictions on the total number of deaths over a time-window of 104 days from the beginning of the simulation (4th February) to the relaxation of the more severe NPIs (18th May). We plot the two basis matrices for three different intervention scenarios. In (a,b), both mobility restrictions and activity reduction are applied as per the actual application dates. In (c,d), hypothetical 15-days early implementation of both strategies. In (e,f), mobility restrictions are enacted even earlier, on 4th February, while activity reduction is applied 15 days in advance with respect to its actual implementation. In (b,d,f), we show the Province's weights related to the two basis matrices, coloured respect to the results of the k-means algorithm. This figure extends Fig. 6 in the main document, which shows two exemplary Provinces.

# S5 Further details on the uplifting timing of NPIs

Figure S3 provides insight on the scenarios of uplifting of NPIs, with details on the two exemplary Provinces of *Sud Sardegna* (panels (a)–(c)) and *Bergamo* (panels (d)–(f)) and at the National level (panels (g)–(i)).

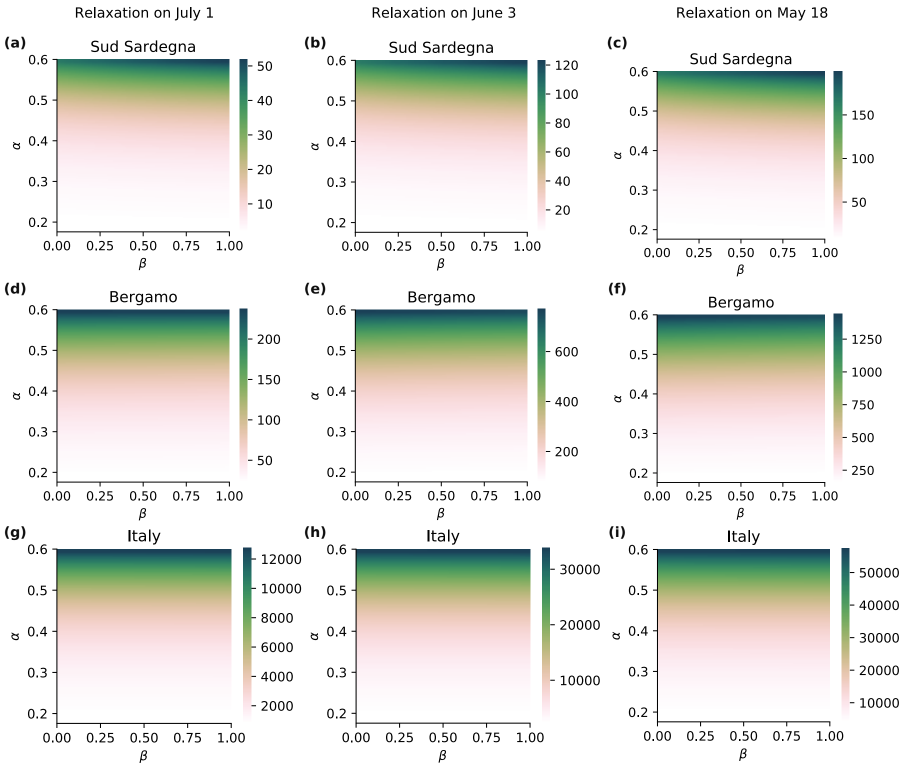


Figure S3: Effect of the relaxation of NPIs, for different post-relaxation levels of activity reduction and mobility restrictions. We consider the number of deaths over a time-window of 60 days from the relaxation date for three different scenarios. In (a,d,g), we consider a late hypothetical uplift of the restrictions on July 1. In (b,e,h), we consider as relaxation date June 3, which corresponds to the complete relaxation of mobility restrictions in Italy. In (c,f,i), we consider as relaxation date 18th May, corresponding to the first uplifting of NPIs in Italy. In (a–f), we report the results for two Provinces that have shown different responses in the implementation of NPIs: (a–c) *Sud Sardegna* and (d–f) *Bergamo*. In (g–i), we show the results aggregated at the country. This figure provides further details to Fig. 8 of the main document, which only contains panels (c,f,i).

# S6 NMF to analyse the uplifting of mobility restrictions

NMF was utilised to perform similar what-if analyses on the scenarios of relaxation of NPIs. Results are illustrated in Fig. S4. In all the considered scenarios, the first component explained most of the variations, due to the smaller values of the entries of matrix $C_2$ and of the corresponding weights. As a result, travel restrictions are unlikely to have a primary effect during relaxation of NPIs.

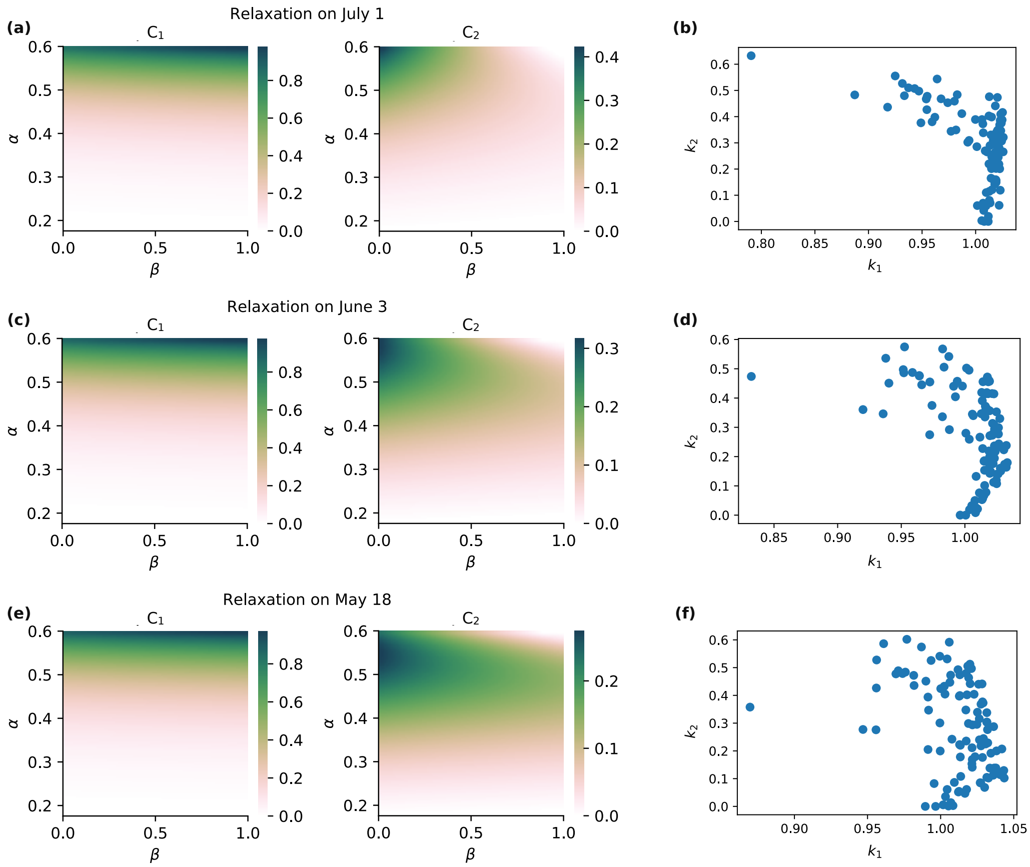


Figure S4: Effect of the relaxation of NPIs, for different post-relaxation levels of activity reduction and mobility restrictions. We consider the number of deaths over a time-window of 60 days, and we show the two basis matrices for three different scenarios. In (a,b), we show a late hypothetical relaxation of the restrictions on 1st July. In (d,c), we consider as relaxation date 3rd June, which corresponds to the complete relaxation of mobility restrictions in Italy. In (e,f), we consider as relaxation date 18th May, corresponding to the first uplifting of NPIs in Italy. In (b,d,f), we show the Provinces' weights related to the two basis matrices.

# S7 Additional supporting simulations and figures

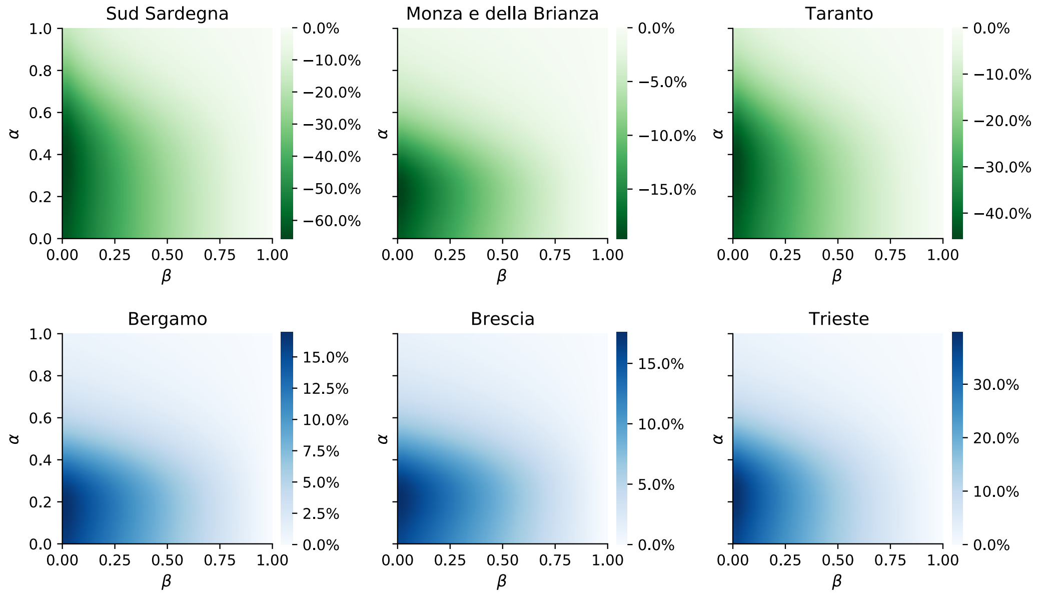


Figure S5: Effect of early application of mobility restrictions. We consider the total number of deaths over a time-window of 104 days from the beginning of the simulations (4th February) to the time corresponding to the relaxation of the most severe NPIs in Italy (18th May). We plot different combinations of levels of activity reduction and mobility restrictions, implemented on 5th March (actual date) and 4th February (early implementation), respectively. For each level of activity reduction $\alpha$ (row of the heat-map), the effect of mobility restrictions is reported in terms of the percentage difference in the total number of deaths with respect to the corresponding case with no mobility restrictions ($\beta = 1$). We show the results for six Provinces, selected as representative examples. This figure extends the results illustrated in Fig. 5 of the main document, which reports predictions aggregated at the country level.

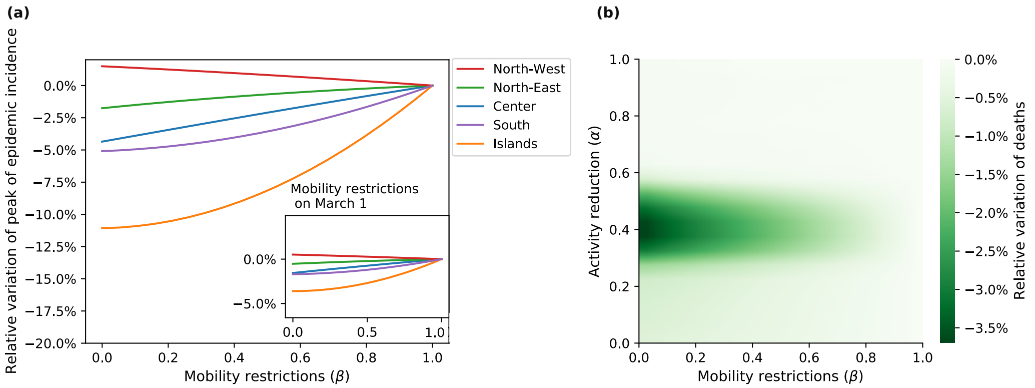


Figure S6: Effect of early application of mobility restrictions on the peak of the epidemic incidence. We consider the maximum number of new infected individuals from the beginning of the simulations (4th February) to the time corresponding to the relaxation of the most severe NPIs (18th May). In (a), we consider the effect of different levels of mobility restrictions enacted on 4th February (almost one month earlier than the actual dates). The figure inset shows the effect of the same interventions applied on March 1 (the actual application date in North Italy). The activity reduction parameter is fixed to the lockdown level $\alpha_{\text{low}} = 0.176$. Results are aggregated at the macro-region level and reported as the variation of the infected individuals at the peak of the epidemic incidence $C_{\text{peak}}$, with respect to the case with no mobility restrictions ($\beta = 1$). In (b), we consider different combinations of levels of activity reduction and mobility restrictions, implemented on 5th March (actual date) and 4th February (early implementation), respectively. For each level of activity reduction $\alpha$ (row), the effect of mobility restrictions is reported in terms of the percentage difference in the number of infected individuals at the peak of the epidemic incidence with respect to the corresponding case with no mobility restrictions ($\beta = 1$).

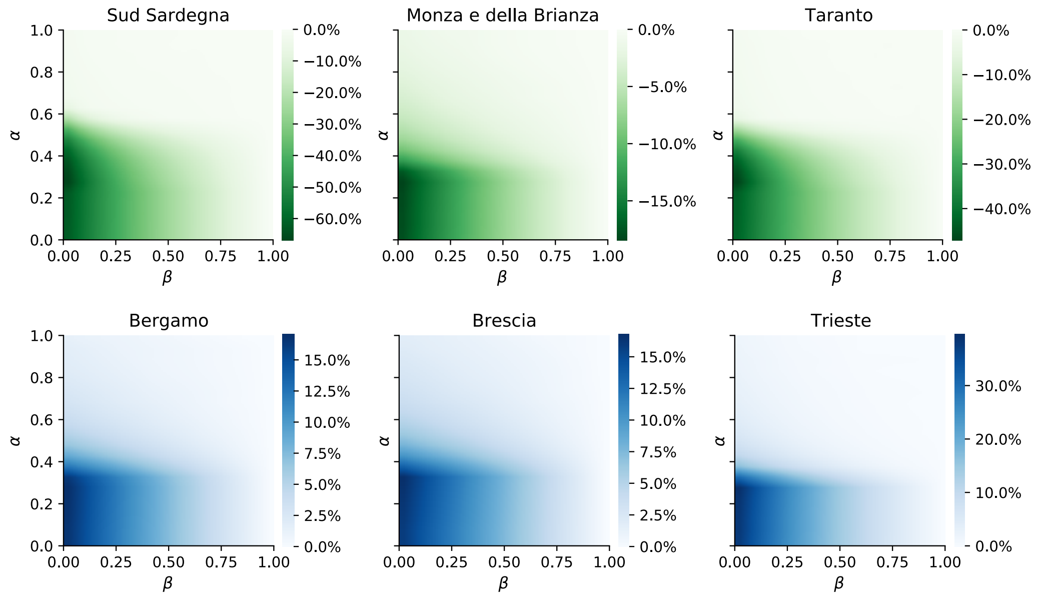


Figure S7: Effect of early application of mobility restrictions on the peak of the epidemic incidence for six Provinces, selected as representative examples. We consider the maximum number of new infected individuals from the beginning of the simulations (4th February) to the time corresponding to the relaxation of the most severe NPIs (18th May). We consider different combinations of levels of activity reduction and mobility restrictions, implemented on 5th March (actual date) and 4th February (early implementation), respectively. For each level of activity reduction $\alpha$ (row), the effect of mobility restrictions is reported in terms of the percentage difference in the number of infected individuals at the peak of the epidemic incidence with respect to the corresponding case with no mobility restrictions ($\beta = 1$).

# Supplementary references


[1] COVID-19 Italia - Monitoraggio situazione. GitHub; 2020. Accessed: October 30, 2020. https://github.com/pcm-dpc/COVID-19.

[2] Gazzetta Ufficiale. Gazzetta Ufficiale della Repubblica Italiana; 2020. Accessed: October 30, 2020. Available at https://www.gazzettaufficiale.it.

[3] Jain AK, Murty MN, Flynn PJ. Data clustering: a review. ACM Computing Surveys. 1999;31(3):264–323. doi:10.1145/331499.331504.
